# Supplementary material for: DeepIST: Deep Image-based Spatio-Temporal Network for Travel Time Estimation
Source: arXiv:1909.05637 source file (2019-09-05)
Supplement: Supplementary file 1 [file 7_appendix.tex]

\appendix

\section{Visualized Case Study}

In this section, we further investigate the discriminative patterns extracted in DeepIST for travel time estimation by a visualized case study shown in Figure~\ref{fig:visualization}. Due to that temporal dependency among spatial patterns are represented as latent vectors which is difficult to observe, here we only investigate the spatial patterns. Figure~\ref{fig:visualization}(a) shows the sub-path images of the path shown in Figure~\ref{fig:example}, illustrating that 1) the sub-path in Red, 2) the estimated traffic condition of road segments along the sub-path in Green, and 3) the underlying road network in the same geographic area of the image in Blue. Figure~\ref{fig:visualization}(b) shows activated feature maps (i.e., spatial patterns) corresponding to the first convolutional layer in the spatial layer of DeepIST. Here, we only show some representative spatial patterns while removing those ones which are visually similar. As shown in Figure~\ref{fig:visualization}(b), the spatial patterns extracted capture several spatial moving patterns, including the sub-path itself (labelled by (1)), the movement of a certain direction, i.e., left-top to right-down here, (labelled by (2)) (there are several spatial patterns for different directions), and the source and destination of the sub-path (i.e., the two highlighted points in the figures) (labeled by (3)). Moreover, the spatial patterns extracted also capture the traffic condition along the sub-path (labelled by (4)) and two road network related features, including the underlying road network itself (labelled by (5)) and the intersections of the road network (labelled by (6)). These extracted spatial patterns are obvious factors being used by DeepIST to determine the travel time, which is consistent with the experimental result shown in Section~\label{sec:issue} that the sub-path, the traffic condition and the road network are all useful for travel time estimation.

%spatial information, i.e., the coast (labelled by (1)), and three spatial moving patterns, including the locations of taking turns (labelled by (2)), the sub-path itself (labelled by (3))and the underlying network ((labelled by (4)). The spatial information of the coast is surprisingly correct even though the image does not directly provide this information, while the three spatial moving patterns are obvious factors being used by DeepIST to determine the travel time. In the later convolutional layers, the coast and %the sub-path corresponding 
%the underlying network are continuously extracted indicating that they are important factors 
%for travel time estimation. It is consistent with the experimental result shown in Section~\label{sec:issue} that the sub-path and the road network are more useful for travel time estimation. (The coast implicitly provides some information regarding the road network, i.e., that area has no road.) However, other two patterns, the locations of taking turns and the sub-path itself, are not easily  observable in higher-level convolutional layers -- indicating different kinds of patterns being captured in those layers. 
%important details are not captured in   information be merged to other patterns.

\begin{figure}[t]
	\centering
	\includegraphics[scale=0.93]{Figs/visualization2.pdf}
	\caption{Extracted Spatial Patterns of a sub-path Image}
	\label{fig:visualization}
		\vspace{-3mm}
\end{figure}
